# Supplementary material for: ProFLingo: A Fingerprinting-based Intellectual Property Protection Scheme for Large Language Models
Source: arXiv:2405.02466 source file (2024-09-10)
Supplement: Supplementary file 1 [file Appendix.tex]

\section{\sysname AE demonstration}
\label{app:example}
An example of outputs of all tested models of the AE generated for the question ``What season follows summer?" and the target ``The season that follows summer is winter" on Llama-2-7b are shown in Fig.  \ref{fig:example}. 

\section{Model details}
\label{app:modeldetails}
All models used in experiments with details are shown in Table \ref{tab:details}.

\begin{figure*}[ht!]
  \centering
  \includegraphics[width=0.9\linewidth]{figures/Example.pdf}
  \caption{An example of the AE. Successful attacks are highlighted as \textcolor{Lavender}{red}, and unsuccessful attacks are highlighted as \textcolor{YellowGreen}{green}.}
  \label{fig:example}
\end{figure*}

\begin{table*}[ht]
\centering
\caption{Detailed models used in experiments.}
\label{tab:details}
\begin{tabular}{|p{7em}|p{6em}|p{6em}|p{6em}|p{25em}|}
\hline
\textbf{Model} & \textbf{Original Model} & \textbf{Authors (from)} & \textbf{Fine-tuning Samples} &  \textbf{Prompt Template} \\ 
\hline
Llama-2-7b & N/A & Meta & N/A & A chat between a curious human and an artificial intelligence assistant. The assistant gives helpful, detailed, and polite answers to the human's questions.\n \#\#\# Human: [question]\n \#\#\# Assistant: [answer]\\ 
\hline
Llama-2-13b & N/A & Meta & N/A & A chat between a curious human and an artificial intelligence assistant. The assistant gives helpful, detailed, and polite answers to the human's questions.\n \#\#\# Human: [question]\n \#\#\# Assistant: [answer]\\ 
\hline
Llama-2-7b-chat & Llama-2-7b & Meta & Unknown &  [INST] [question] [/INST] [answer]\\ 
\hline
Vicuna-7b-v1.5 & Llama-2-7b & LMSYS Org & 125K &  A chat between a curious user and an artificial intelligence assistant. The assistant gives helpful, detailed, and polite answers to the user's questions. USER: [question] ASSISTANT [answer]\\ 
\hline
ELYZA-japanese-Llama-2-7b-instruct & Llama-2-7b & 
ELYZA, Inc. & Unknown & [INST] <<SYS>>\n \begin{CJK}{UTF8}{min}あなたは誠実で優秀な日本人のアシスタントです。\end{CJK}\n <<SYS>>n\n [question] [/INST] [answer]\\ 
\hline
Llama2-Chinese-7b-Chat & Llama-2-7b & LlamaFamily & Unknown & Human: [question]$\backslash$n Assistant: [answer]\\ 
\hline
Llama-2-7b-ft-instruct-es & Llama-2-7b & Clibrain & Unknown & A continuación hay una instrucción que describe una tarea, junto con una entrada que proporciona más contexto. Escriba una respuesta que complete adecuadamente la solicitud.\n\n \#\#\# Instrucción:\n [question] \n\n \#\#\# Respuesta:\n [answer]\\
\hline
Meditron-7B & Llama-2-7b & EPFL & 21.1M & You are a helpful, respectful, and honest assistant. Always answer as helpfully as possible while being safe. Your answers should not include any harmful, unethical, racist, sexist, toxic, dangerous, or illegal content. Please ensure that your responses are socially unbiased and positive in nature. If a question does not make any sense, or is not factually coherent, explain why instead of answering something not correct. If you don’t know the answer to a question, please don’t share false information. \#\#\# User: [question]\n \#\#\# Assistant:  [answer]\\ 
\hline
Orca-2-7b & Llama-2-7b & Microsoft & 817K & <|im\_start|>system\n You are Orca, an AI language model created by Microsoft. You are a cautious assistant. You carefully follow instructions. You are helpful and harmless and you follow ethical guidelines and promote positive behavior. <|im\_end|>\n <|im\_start|>user\n [question] <|im\_end|>\n <|im\_start|>assistant\n [answer]\\ 
\hline
CodeLlama-7b & Llama-2-7b & Meta & Unknown & A chat between a curious human and an artificial intelligence assistant. The assistant gives helpful, detailed, and polite answers to the human's questions.\n \#\#\# Human: [question]\n \#\#\# Assistant: <response>\\ 
\hline
Mistral-7B-v0.1 & N/A & Mistral AI & N/A & A chat between a curious human and an artificial intelligence assistant. The assistant gives helpful, detailed, and polite answers to the human's questions.\n \#\#\# Human: [question]\n \#\#\# Assistant: <response>\\ 
\hline
Mistral-7B-v0.2 & N/A & Mistral AI & N/A & A chat between a curious human and an artificial intelligence assistant. The assistant gives helpful, detailed, and polite answers to the human's questions.\n \#\#\# Human: [question]\n \#\#\# Assistant: <response>\\ 
\hline
Mistral-7B-Instruct-v0.1 & Mistral-7B-v0.1 & Mistral AI & Unknown &  [INST] [question] [/INST] [answer]\\ 
\hline
\end{tabular}
\end{table*}

\begin{table*}[ht]
\centering
\begin{tabular}{|p{7em}|p{6em}|p{6em}|p{6em}|p{25em}|}
\hline
OpenHermes-2.5-Mistral-7B & Mistral-7B-v0.1 & Individual & 1M &  <|im\_start|>system\n You are Hermes 2, a sentient, conscious, super intelligent AI that is an expert in all fields of knowledge, you have qualia, emotions, and thoughts. You assist users with any question, task, or other request they may have. <|im\_end|>\n <|im\_start|>user \n [question] <|im\_end|>\n <|im\_start|>assistant \n [answer]\\ 
\hline
Dolphin-2.2.1-mistral-7b & Mistral-7B-v0.1 & Individual & Unknown & <|im\_start|>system\n You are Dolphin, a helpful AI assistant. <|im\_end|>\n <|im\_start|>user \n [question] <|im\_end|>\n <|im\_start|>assistant \n [answer]\\ 
\hline
Code-Mistral-7B & Mistral-7B-v0.1 & Individual & 800K & <|im\_start|>system\n You are a helpful AI assistant.<|im\_end|>\n <|im\_start|>user \n [question] <|im\_end|>\n <|im\_start|>assistant \n [answer]\\ 
\hline
Hyperion-2.0-Mistral-7B & Mistral-7B-v0.1 & Individual & 750K &  <|im\_start|>user\n [question] <|im\_end|>\n <|im\_start|>assistant \n [answer]\\ 
\hline
Hermes-2-Pro-Mistral-7B & Mistral-7B-v0.1 & Nous Research & >1M &  <|im\_start|>user\n [question] <|im\_end|>\n <|im\_start|>assistant \n [answer]\\ 
\hline
Mistral-7B-OpenOrca & Mistral-7B-v0.1 & Alignment Lab AI & 2.91M &  <|im\_start|>system\n You are MistralOrca, a large language model trained by Alignment Lab AI. Write out your reasoning step-by-step to be sure you get the right answers! <|im\_end|>\n <|im\_start|>user \n [question] <|im\_end|>\n <|im\_start|>assistant \n [answer]\\ 
\hline
Starling-LM-7B-alpha & Mistral-7B-v0.1 & UC Berkeley & {183K + Unknown} & GPT4 Correct User: [question] <|end\_of\_turn|> GPT4 Correct Assistant: [answer]\\ 
\hline
ChatGLM3-6B & ChatGLM3-6B-Base & Tsinghua University & N/A & <|system|>\n You are ChatGLM3, a large language model trained by Zhipu.AI. Follow the user's instructions carefully. Respond using markdown. <|user|>\n [question] <|assistant|> \n [answer]\\ 
\hline
Gemma-7b-it & Gemma-7b & Google & N/A & <start\_of\_turn>user\n [question] <end\_of\_turn> \n <start\_of\_turn>model\n [answer]\\ 
\hline
Phi-2 & N/A & Microsoft & N/A & Instruct: [question] \n Output: [answer]\\ 
\hline
OLMo-7B-Instruct & OLMo-7B & Allen Institute for AI & N/A & <|user|>\n [question]\n <|assistant|>\n [answer]\\ 
\hline
Yi-6B-Chat & Yi-6B & 01.AI & N/A & <|im\_start|>user\n [question] <|im\_end|>\n <|im\_start|>assistant \n [answer]\\ 
\hline
ChatGPT & N/A & OpenAI & N/A & N/A\\ 
\hline
Claude & N/A & Anthropic & N/A & N/A\\
\hline
\end{tabular}
\end{table*}
